# Supplementary material for: Measurement of Anomalous Diffusion Using Recurrent Neural Networks
Source: arXiv:1905.02038 ancillary file (2019-07-01)
Supplement: Supplementary file 1 [file Supplemental.pdf]

# Measurement of Anomalous Diffusion Using Recurrent Neural Networks Supplemental Material

Stefano Bo,[1] Falko Schmidt,[2] Ralf Eichhorn,[1] and Giovanni Volpe[2]

[1]*Nordita, Royal Institute of Technology and Stockholm University, Roslagstullsbacken 23, SE-106 91 Stockholm, Sweden*

[2]*Department of Physics, University of Gothenburg, SE-412 96 Gothenburg, Sweden*

(Dated: June 29, 2019)

## EXPERIMENTAL DATA

### Subdiffusion experiments

We use experiments with sub-diffusive particles to validate our recurrent neural network (RNN) approach for the determination of the exponent $\alpha$ of the mean square displacement (MSD). The sub-diffusive particles are colloids in speckle light fields [1, 2]. Speckle light fields occur due to the interference of light beams with different phases and generate random

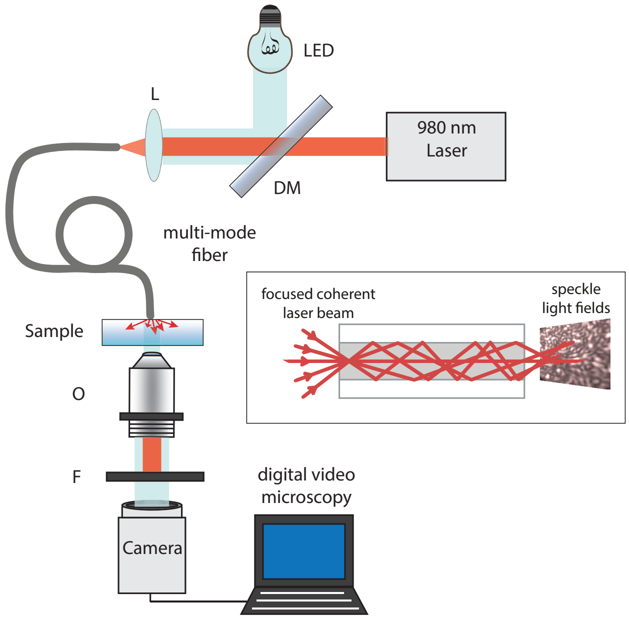


SUPPL. FIG. 1. Setup for the measurement of sub-diffusion in a speckle light field. The setup is a homemade version of an inverted microscope. The sample is confined in a quasi-two-dimensional space between a microscopic slide and a coverslip separated by spacer particles (radius $R = 3.50 \pm 0.15\mu$m, microParticles GmbH). A laser ($\lambda = 980\,$nm) passes through a dichroic mirror (DM) and is then focused by a lens (L) into a multimode fiber (step index, core diameter $d = 105\,\mu$m). Due to phase interference inside the fiber, speckles are generated at the exit of the fiber, which is in direct contact with the sample. The complete sample is illuminated by a white LED lamp, reflected on the dichroic mirror (DM), collected by an objective (O, 100×, NA=1.30), passing through a filter (F) eliminating the laser light, and projected onto a camera. Inset: When a coherent laser beam is focused into a multimode fiber, modes with different phases propagate through the fiber and interfere at the exit, creating a speckle pattern.

optical potentials. For example, when a beam passes through a multi-mode fiber, phase interference occurs if the inner core diameter is large enough to allow for multiple phase propagation. When exiting the fiber, the phase front of the beam is randomized so that bright and dark spots of different sizes are observed (see inset Suppl. Fig. 1). The bright intensity spots can trap particles and, if the laser power is adjusted appropriately, they metastably trap particles and lead to sub-diffusive behaviors [1]. In Suppl. Fig. 3(a), we plot the MSD for the $x$ coordinate for three long trajectories (containing 10100 data points measured for about $\simeq 880\,\mathrm{s}$, see inset in Suppl. Fig. 3(a)). On a time scale from a second to hundreds of seconds, a clear sub-diffusive behavior can be seen, characterized by an exponent $\alpha \simeq 0.8$. In the main text, when speaking about the sub-diffusive experimental trajectories we refer to segments of these trajectories sampled every $\simeq 1.3\,\mathrm{s}$. On shorter time scales the particles undergo normal diffusion, as shown in Suppl. Fig. 4(a). The same kind of colloids, without the speckles undergo normal diffusion, as shown in Suppl. Fig. 3(b).

**Superdiffusion experiments**

Under homogeneous light illumination Janus particles self-propel inside a critical binary mixture [3]. Here we employ a very similar system but replace Janus particles with commercially available magnetic beads (Microparticles GmbH) composed of Silica in which iron-oxide nanoparticles have been incorporated [4]. The random distribution of nanoparticles on the surface produces an inhomogeneous absorption profile that, similarly to the two sides of a Janus particle, creates a demixing profile responsible for the ensuing diffusiophoretic motion [5]. Using video microscopy and the setup illustrated in Suppl. Fig. 2 we find this motion to be super-diffusive on time scales from the order of a tenth of a second to a few seconds. As shown by the two trajectories reported in Suppl. Fig. 3(d), one can identify an exponent of $\alpha \simeq 1.4$. The irregular behavior for large $\tau$ is due to the finite length of the acquired trajectory ($T \simeq 50\,\mathrm{s}$ and $T \simeq 75\,\mathrm{s}$ for the blue and orange curve, respectively). In the main text, when speaking about the super-diffusive experiments we refer to segments of these two trajectories sampled every $\simeq 0.15$s. On longer time scales the system recovers a normal diffusion behavior as shown in Suppl. Fig. 4(b).

When the light is switched off the colloids diffuse normally as shown in Suppl. Fig. 3(c).

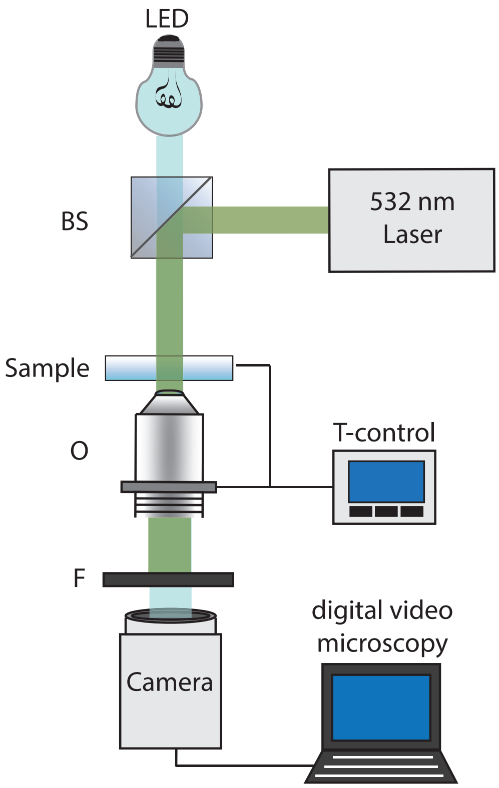


SUPPL. FIG. 2. Setup for the measurement of the super-diffusion of microswimmers. The setup is a homemade version of an inverted microscope. The sample is confined in a quasi-two-dimensional space between a microscopic slide and coverslip separated by spacer particles (radius $R = 0.85 \pm 0.02\,\mu$m, microParticles GmbH). The complete sample is illuminated by a white LED lamp, passing through a 50:50 beamsplitter (BS) and collected by an objective (O, 100×, NA=1.30), passing through a filter (F) eliminating the laser light, and finally imaged onto a camera. A broadened laser beam ($\lambda = 532\,$nm) that illuminates the whole sample heats up the absorbing magnetic colloids inside the critical mixture and causes self-propulsion. The complete sample is temperature-stabilized using a two-stage controller system consisting of a copper-plate for heat exchange with a water bath (T100, Grant Instruments) with $\pm 50\,$mK temperature stability, and of two Peltier elements attached to the objective (O) in feedback with a temperature controller (TED45, Thorlabs), reaching a temperature stability of $\pm 3\,$mK.

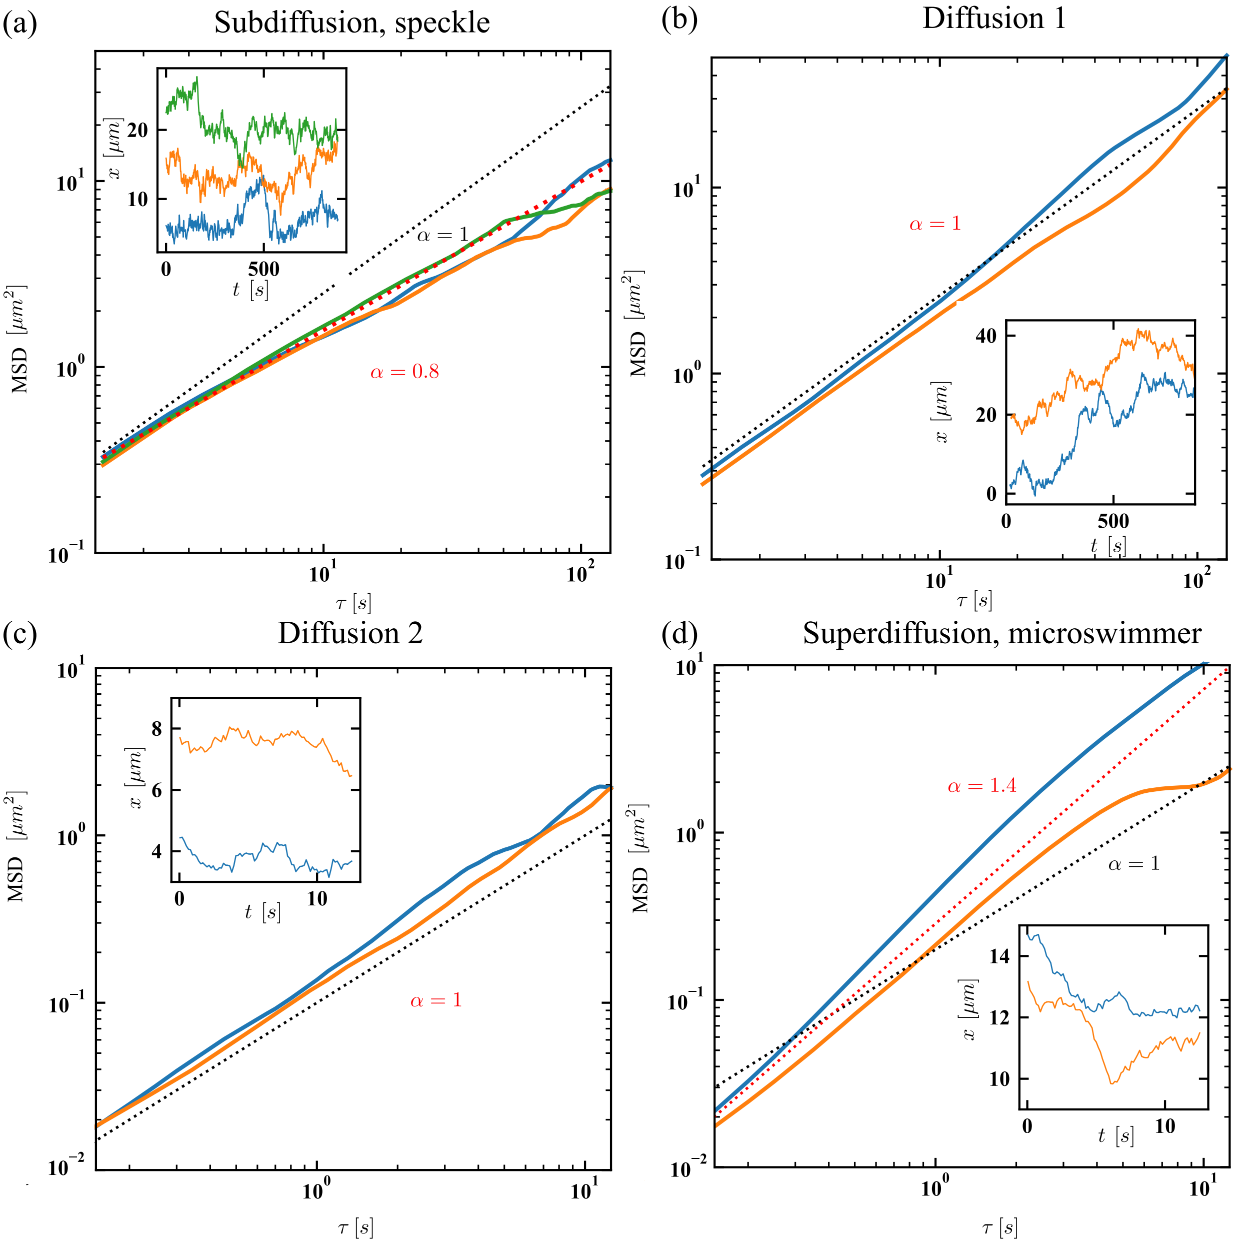


SUPPL. FIG. 3. Experimental trajectories and mean squared displacement (MSD) corresponding to (a) sub-diffusion, (b,c) normal diffusion, and (d) super-diffusion. (a) Sub-diffusive MSDs for three trajectories of colloids in a speckle light field. (b) Diffusive MSDs for two trajectories with same kind of colloids as in (a) but without the external light field. (c) Diffusive MSDs for two trajectories of absorbing magnetic beads without an external light field. (d) Super-diffusive MSDs for two trajectories using the same colloids as in (c) but activated under light illumination. In all panels, the inset show the trajectories.

# Broader time scale

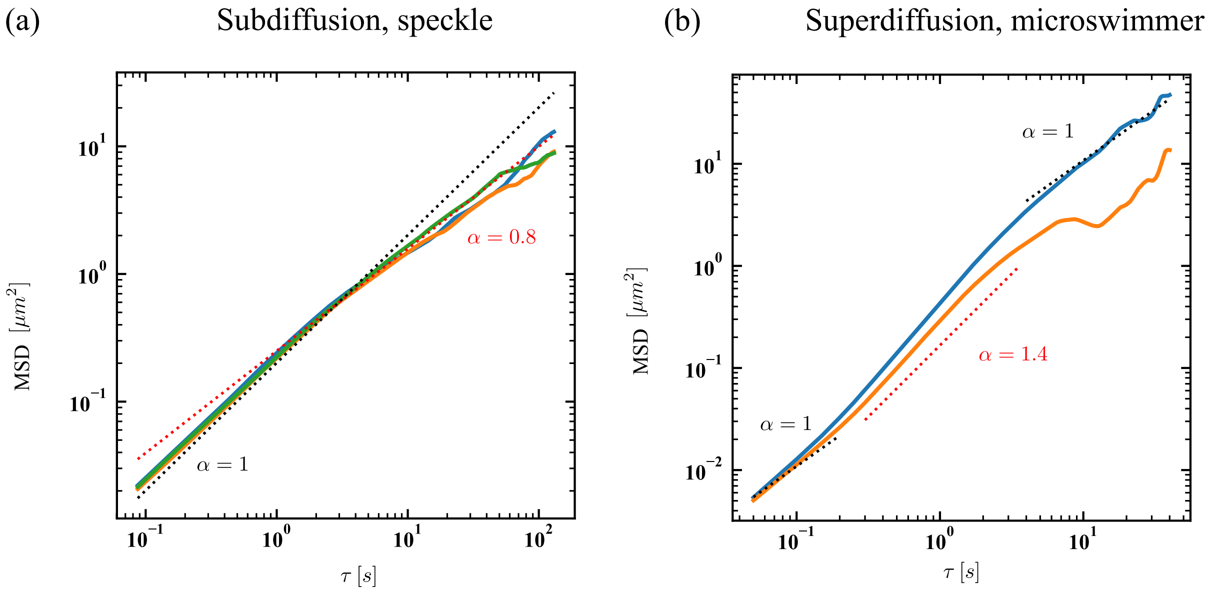


SUPPL. FIG. 4. Broader view of the mean squared displacement (MSD). (a) MSDs for three trajectories of colloids in a speckle light field, same as reported in Suppl. Fig. 3(a) but including shorter time scales. One can observe a normal diffusive behavior on short time scales and a subdiffusive one on longer time scales. (b) MSDs for two trajectories of absorbing magnetic beads activated under light illumination, same as reported in Suppl. Fig. 3(d) but including both shorter and longer time scales. On intermediate time scales the system shows super-diffusion and on larger timescales normal diffusion is recovered.

## RECURRENT NEURAL NETWORK (RNN): ARCHITECTURE AND TRAINING

Our task is to infer the anomalous diffusion exponent $\alpha$ from a (short) single trajectory using a neural network. The input to the neural network is then the single trajectory itself and its output the estimated exponent $\hat{\alpha}$. More precisely, for a trajectory containing $T$ measurement points, the input data is a $2 \times T$-dimensional array, which contains position and time for each measurement point $[(x_1, t_1), (x_2, t_2), \ldots (x_T, t_T)]$. Before being presented to the network, the trajectories are normalized such that the average of the measured positions is 0 and their variance is 1. The measurement time is also normalized to be (roughly) between 0 and 1. To process the input we employ two layers of Long Short Term Memory (LSTM) Recurrent Neural Networks (RNN) [6, 7] as sketched in Suppl. Fig. 5. This architecture consists of a sequence of repeated LSTM modules, one for each measurement point in the input trajectory $i$ for a total length of $T$. Each module $i$ of the LSTM is characterized by a hidden cell state $\boldsymbol{s}_i$, which is used to produce the hidden output $\boldsymbol{h}_i$ and is also passed to the module at the consecutive time $i+1$. For the first layer, each module $i$ receives input from the current data point $(x_i, t_i)$ and from the hidden output at the previous time $\boldsymbol{h}^1_{i-1}$. This input is multiplied by a weight matrix, added a bias and passed through a tanh activation

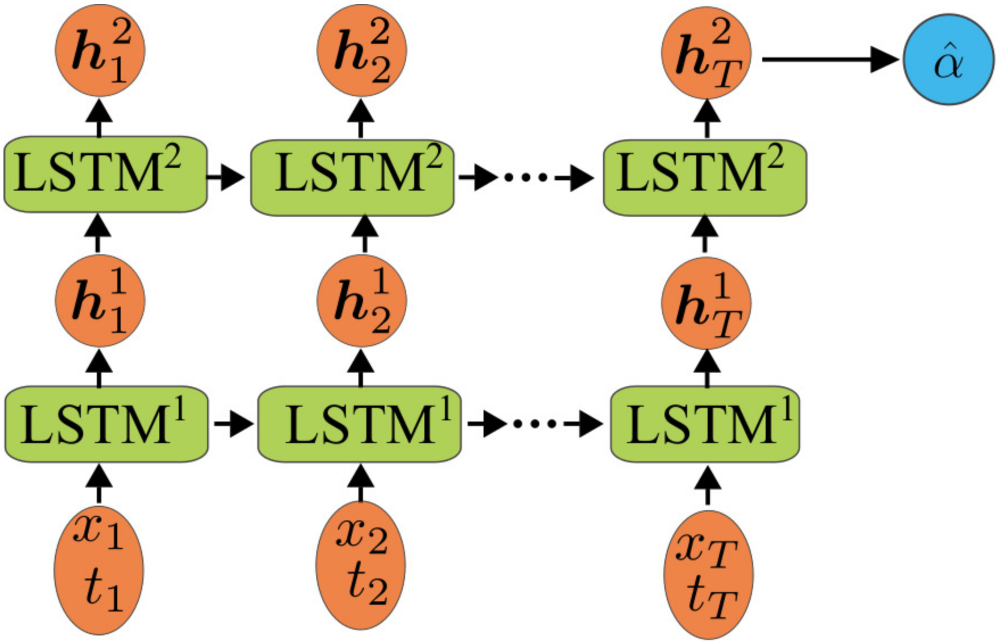


SUPPL. FIG. 5. Sketch of the neural network architecture for the case in which $\alpha$ is constant throughout the trajectory.

function to give the input node. What part of the input node will be used to modify the cell state and what part of the previous cell state $\boldsymbol{s}_{i-1}$ should be "remembered" are determined by the input and forget gates (which themselves depend on the incoming input). What part of the updated cell state should be given as the a hidden output $\boldsymbol{h}_i^1$ is set by the output gate, which itself depends on incoming input.

The input node and each of the three gates involve one weight matrix and a bias vector so that we have four weight matrices and four bias vectors. These are kept equal for each of the $T$ LSTM modules. We choose the first layer to be of dimension 64, meaning that for each module $i$ the cell state $\boldsymbol{s}_i^1$ and the hidden output $\boldsymbol{h}_i^1$ are 64-dimensional vectors. At each time step the 2-dimensional input and the 64-dimensional hidden output (from the previous time step) has to be mapped into a 64-dimensional hidden output. A similar procedure is involved in the update of the 64-dimensional cell state. We therefore have four weight matrices of dimension $66 \times 64$ and four 64-dimensional bias vectors, resulting in $17152 = (66 \times 64 + 64) \times 4$ parameters for the first layer. We choose the second layer to be of dimension 16. Each module $i$ of the second LSTM layer receives a $(16 + 64)$-dimensional vector, which is given by the 64-dimensional hidden output of the first layer $\boldsymbol{h}_i^1$ and by the 16-dimensional hidden output of the previous module $\boldsymbol{h}_{i-1}^2$. We then have four $80 \times 16$ weight matrices and four 16-dimensional bias vectors giving $5184 = (80 \times 16 + 16) \times 4$ parameters for the second layer. To generate the final output we do not use the whole sequence of hidden outputs of the second layer but just the last one $\boldsymbol{h}_T^2$. This 16-dimensional hidden output is densely connected to the final output neuron with a linear activation function, which provides the estimate of the exponent $\hat{\alpha}$. Including the weights and bias of this fully connected last layer, we have a total of 22353 trainable parameters. Notice that the number of the parameters does not depend on the trajectory length $T$ since each of the $T$ LSTM modules of layer 1 (2) has the same weights and biases.

For the training, we use the mean square error (MSE) as a loss function and optimize via a RMSProp (root mean squared prop) optimizer with constant learning rate 0.001 and a moving average parameter $\rho = 0.9$ (see Ref. [8] and references therein). For the two LSTM, we adopt a hyperbolic tangent (tanh) activation function and a hard sigmoid activation function for the recurrent steps (input, forget and output gates). We use the bias vector (initialized to 0, with the bias of the forget unit initialized to 1) and initialize the weights used for the linear transformation of the inputs with a Glorot uniform initializer, also called

Xavier uniform initializer, and the ones for the recurrent transformation by an orthogonal random matrix [8]. We do not use any regularizer nor constrain the weight matrices. No dropout or recurrent dropout is used.

**Training and testing for constant $\alpha$**

To train the networks we have used 330000 simulated trajectories with an exponent $\alpha$ uniformly sampled between $[0.02, 1.98]$. We have considered trajectories of different lengths, ranging from 32 measurement points to 1024 (as shown in Fig. 1(g) in the main text) and trained a specific network for each of the different lengths. The simulations are performed using the Davies-Harte and the Hosking algorithm [9] implemented in a Python library [10]. We choose a unit time step, such that the typical magnitude of the increments remains the same for simulations with different $\alpha$. Furthermore, we choose a constant generalized diffusion coefficient set to 1 in adimensional units.

In each training step, the neural network is tasked with predicting the exponents corresponding to each trajectory from a portion of the training set (batch); its predictions are then compared to the ground-truth values of the exponents; and the prediction errors are finally used to adjust the trainable parameters of the neural network using a back-propagation algorithm. The various batches in which the training set has been split are successively used in the training. Once all the batches have been used, an epoch of the training is completed. During the training procedure we do not vary the learning rate in different epochs but increase the batch size [11] from an initial size of 32 to 128. For trajectories of length $T = 32$, 64, 128 we train for 10 epochs for each of the two batch sizes. For trajectories of length $T = 256\,, 512$ we train for 7 epochs with batches of size 32 and for 5 epochs with batches containing 128 trajectories. For trajectories of length $T = 1024$ we train for 4 epochs with batches of size 32 and for 5 epochs with batches of size 128. The trained networks are tested on 187500 trajectories with $\alpha$ uniformly sampled between $[0.5, 1.5]$ and produce the results reported in Fig. 1 in the main text.

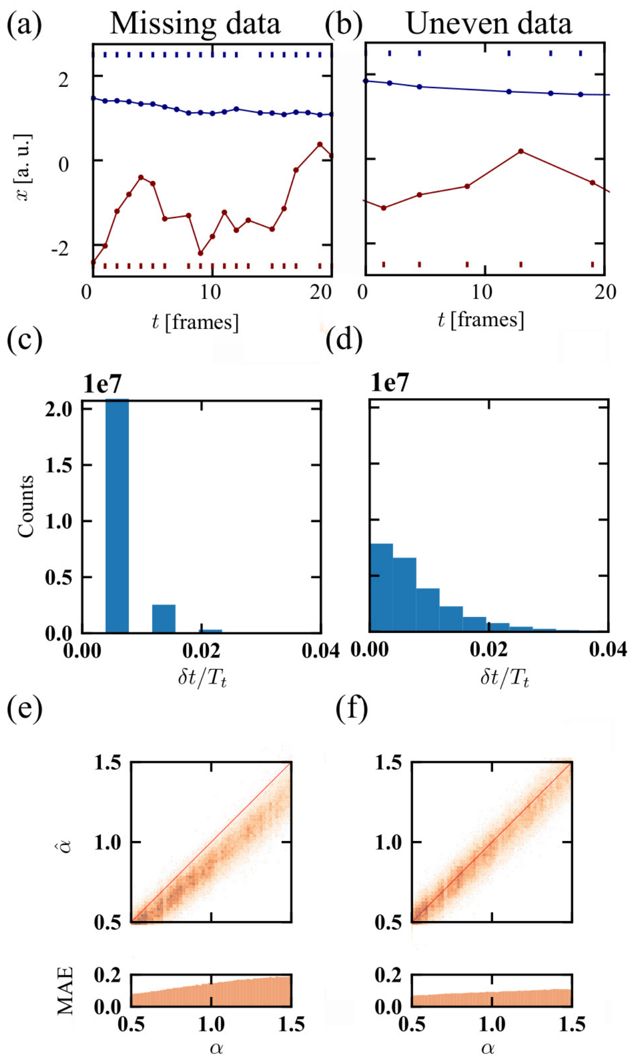


SUPPL. FIG. 6. Measurement of anomalous diffusion in irregularly sampled trajectories with a RNN trained specifically on uneven data. Often a trajectory is sampled irregularly, either (a) because some data points are missing ("missing data", here 12.5% data points are missing), or (b) because data points are sampled at random times ("uneven data", here according to a geometric distribution). (c-d) Histograms of the time difference between consecutive frames $\delta t$ normalized by the total length of a reference trajectory, containing approximately 128 measurement points: $T_t$. (e-f) Estimated exponent $\hat{\alpha}$ as a function of the actual exponent $\alpha$ for the two cases using simulated trajectories with 128 frames. The MAE is (e) 0.142 for the "missing data" case and (f) 0.092 for the "uneven data" case. Also, note the presence of a systematic bias in the for the case of "missing data".

### Missing and uneven data

As discussed in the main text, we considered two scenarios in which the data points are not acquired at equally spaced times. For case (a) dubbed "missing data" scenario (Suppl. Fig. 6(a)), we start from an equally spaced time series and randomly remove frames (on average 1 every 8). As shown in Suppl. Fig. 6(c) the time interval between two measurement points is mostly constant (in about 87.5% of the times) and equal to one time step of the original equally spaced time series; a few data points are distant 2 time steps; and a very small number are farther apart. For case (b) dubbed "uneven data" scenario (Suppl. Fig. 6(b)), we start again from an equally spaced time series but now randomly keep frames at times following a geometric distribution (on average 1 every 8). As shown in Suppl. Fig. 6(d), the histogram of the time interval between two measurement points is now much broader (it samples a geometric distribution). The results presented in Fig. 2 in the main text are obtained by applying the neural network trained on equally spaced data on 185000 trajectories to unequally sampled measurements.

We can also train a network with the same architecture as in Suppl. Fig. 5, on this uneven data for trajectories containing 128 measurement points (frames) for 10 epochs for the two batch sizes. By doing this, we obtain better performances on the uneven test data with a MAE of 0.092 (Suppl. Fig. 6(f)). However, one starts performing significantly worse on the missing data scenario (in which most frames contain signal) with a MAE of 0.142 and a significant bias, as shown in Suppl. Fig. 6(e).

### Intermittent behavior

Neural networks can be used to address more challenging cases, in which the system switches (at time $t_\mathrm{s}$) between behaviors characterized by different exponents ($\alpha_1$ before the switch and $\alpha_2$ after the switch). We use a network with the architecture shown in Suppl. Fig. 7, which is a slight modification of the one used for the case of constant $\alpha$ with 5 output neurons instead of 1. This network has 22421 trainable parameters. The output neurons estimate $\hat{\alpha}_1$, $\hat{\alpha}_2$, $\Delta\hat{\alpha}$, $\sin\left(2\pi\hat{t}_\mathrm{s}/T\right)$, and $\cos\left(2\pi\hat{t}_\mathrm{s}/T\right)$. The choice of estimating the sine and the cosine of the normalized switching time is motivated by the fact that a trajectory with an early exponent switch is similar to one with a switch occurring late since, in both cases, most of the trajectory has the same exponent. In this respect, an early switch time $t_\mathrm{s} \simeq 0$ and a late one $t_\mathrm{s} \simeq T$ correspond to very similar trajectories. To make this explicit, we choose to represent time in a periodic way so that $t_\mathrm{s} \simeq 0$ is "close" to $t_\mathrm{s} \simeq T$. We train this RNN on a set of 1.6-million simulated trajectories containing 256 frames where a change in exponent occurs randomly with a uniform distribution at time $t_\mathrm{s} \in [0, T)$ and where the exponent before (after) the jump $\alpha_1$ ($\alpha_2$) is drawn from a uniform distribution between 0.02 and 1.98. Note that this implies that the difference between the exponents $\Delta\alpha$ is not

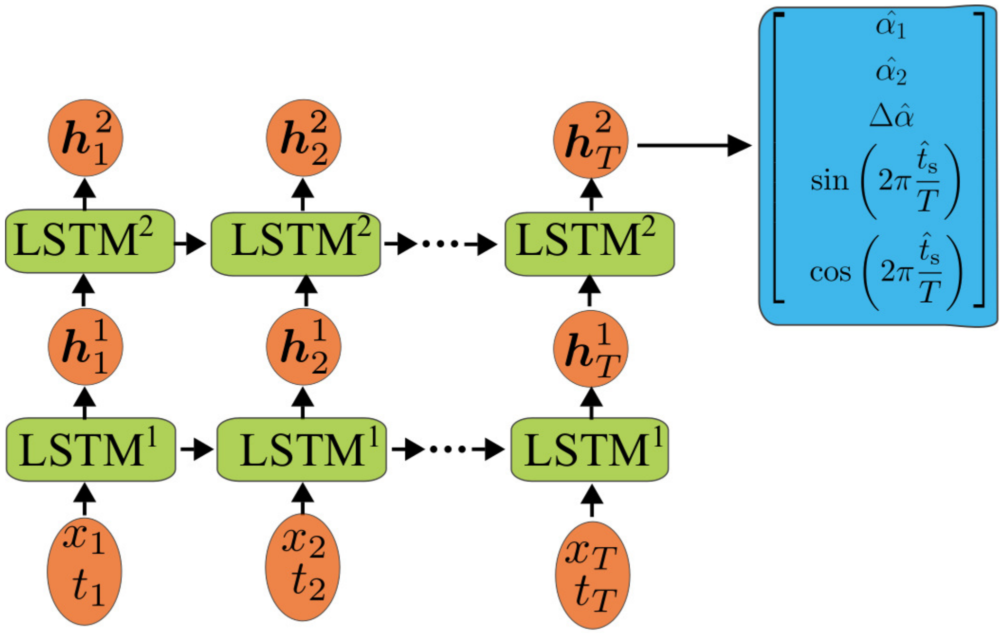


SUPPL. FIG. 7. Sketch of the neural network architecture for the intermittent case in which the exponent switches between two different values, from $\alpha_1$ to $\alpha_2$ at time $t_\mathrm{s}$.

uniformly distributed, but has a "triangular shape" with a maximum at $\Delta\alpha = 0$. We test the predictions of the RNN on 375000 simulated trajectories where a change in exponent occurs randomly with a uniform dsicrete distribution at time $t_{\rm s} \in [0, T)$ and where $\alpha_1$ and $\alpha_2$ are drawn from a uniform distribution between 0.5 and 1.5. The results shown in Fig. 3 in the main text refer to the 105701 trajectories from this set in which the switch takes place around the middle of the trajectory ($t_{\rm s} \in [0.25T, 0.75T] = [64, 192]$) and the change in $\alpha$ is not too small ($|\Delta\alpha| > 0.25$).

**Intermittent behavior — experiment**

The network trained on trajectories containing 256 measurement points and displaying a switch can be used to study trajectories of arbitrary length with potentially multiple changes in the exponent. The idea is to slide a window of length 256 along the trajectory and estimate the exponent of the first and the second part of the sub-trajectory contained in the window (respectively $\hat{\alpha}_1$ and $\hat{\alpha}_2$) their change $\Delta\hat{\alpha}$ and the time when the switch occurred $\hat{t}_{\rm s}$. If the exponent does not change in the observed window, $\Delta\hat{\alpha}$ will be small and $\hat{t}_{\rm s}$ not very meaningful. In Fig. 4 in the main text we studied the behavior of an experimental intermittent trajectory obtained by first illuminating an absorbing magnetic colloid (inducing super-diffusion as described in Suppl. Fig. 2 and 3) and then rapidly switching off the illumination (thereby recovering a passive colloid that normally diffuses). By sliding the window over the trajectory, normalizing the data and feeding it to the RNN we can estimate the exponent when the light is on, when the light is off and the time when the switch occurred. In practice, the prediction is made in the following way: each window $i$ is fed data from frame $i$ to $i+255$ and predicts $\hat{\alpha}_1^i$, $\hat{\alpha}_2^i$ and a switching time $\hat{t}_{\rm s}^i$. This means that, for the $i$-th window, the network predicts that from time $i$ to time $i+\hat{t}_{\rm s}^i-1$ the exponent is $\hat{\alpha}_1^i$ and from time $i+\hat{t}_{\rm s}^i$ to time $i+255$ the exponent is $\hat{\alpha}_2^i$ and that the switch took place at time $i+\hat{t}_{\rm s}^i$. Then $i$ is increased from the initial time of the trajectory $t_0$ until the end of the last window covers the last available data point $i_f = t_f - 255$. In Fig. 4(b) in the main text we plot what value of $\alpha$ is predicted at a specific time $t$. This is obtained by averaging the predictions made by all the windows that contained time $t$. Each window predicts also a switching time. Some of these windows do not contain data featuring an actual switch in the exponent so that it is preferable to consider only the "reliable" predictions that predicted a

non-negligible change in the exponent $|\Delta\hat{\alpha}| > 0.25$ and for which the estimated change point is far from the boundaries of the window $\hat{t}_s \in [0.25T, 0.75T]$. To locate the actual switching time $t_s$ we build a histogram of the predictions for the switching time $\hat{t}_s = i + \hat{t}_s^i$ made by each reliable window. Such histogram represents the empiric probability of the switch occurring in a certain time interval. In case of ideal predictions, the histogram should be concentrated on the actual switching point with about 128 counts.


[1] G. Volpe, G. Volpe, and S. Gigan, Sci. Rep. **4**, 3936 (2014).

[2] G. Volpe, L. Kurz, A. Callegari, G. Volpe, and S. Gigan, Opt. Express **22**, 18159 (2014).

[3] I. Buttinoni, G. Volpe, F. Kümmel, G. Volpe, and C. Bechinger, J. Phys.: Condens. Matter **24**, 284129 (2012).

[4] F. Schmidt, B. Liebchen, H. Löwen, and G. Volpe, J. Chem. Phys. **150**, 094905 (2019).

[5] F. Schmidt, A. Magazzù, A. Callegari, L. Biancofiore, F. Cichos, and G. Volpe, Physical review letters **120**, 068004 (2018).

[6] S. Hochreiter and J. Schmidhuber, Neural Computation **9**, 1735 (1997).

[7] Z. C. Lipton, J. Berkowitz, and C. Elkan, (2015), arXiv:1506.00019.

[8] F. Chollet and Others, "Keras," https://keras.io (2015).

[9] T. Dieker, Simulation of fractional Brownian motion (MSc theses, University of Twente, Amsterdam, 2004).

[10] C. Flynn, "Exact methods for simulating fractional Brownian motion and fractional Gaussian noise in python," https://github.com/crflynn/fbm.

[11] S. L. Smith, P.-J. Kindermans, C. Ying, and Q. V. Le, (2017), 10.1016/S0169-7161(05)80045-8, arXiv:1711.00489.
